# Supplementary material for: Topologies on unparameterised rough path space
Source: arXiv:2407.17828 source file (2024-07-25)
Supplement: Supplementary file 1 [file appendix.tex]

\section{Your Appendix}
This is your appendix.
